# Supplementary material for: High-Frequency Trading on Decentralized On-Chain Exchanges
Source: arXiv:2009.14021 source file (2020-09-29)
Supplement: Supplementary file 1 [file appendix2.tex]

\section{AMM DEX implementations}\label{appendix:uniswap_state_transition_model}
In this section we discuss {\color{red}several} real world AMM DEX implementations.

\subsection{Uniswap}
Uniswap~\cite{uniswap2018} is an AMM DEX on the Ethereum blockchain. Note that the Uniswap model is derived from the generic AMM model, with the following major differences:

\begin{itemize}
    \item Asset $X$ is ETH, and asset $Y$ is an ERC20 asset.
    \item All calculations are performed using integer operations, instead of real number mathematical operations, as Uniswap is implemented on Ethereum.
    \item A $0.3\%$ transaction fee is charged for each liquidity taker transaction ($\text{TransactXForY}(\delta_x)$). In other words, $c_x(\delta_x) = \frac{3}{1000} \delta_x,\ c_y(\cdot) = 0$
    \item For $\text{TransactXForY}(\delta_x)$, a liquidity taker can choose one of the following protections against excessive slippage:
    \begin{itemize}
        \item Fix the input amount $\delta_x$, and specify a minimum $Y$ output amount ($\hat{\delta_y}$).
        \item Fix the output amount $\delta_y$, and specify a maximum $X$ input amount ($\check{\delta_x}$).
    \end{itemize}
    
    \item For $\text{AddLiquidity}(\delta_x, \delta_y)$, the total value of funds deposited into asset $X$ must equal the total value of funds deposited into asset $Y$, according to the exchange rate of the corresponding Uniswap contract. Mathematically, when adding liquidity to an Uniswap contract with a state of $(x, y)$, $\frac{\delta_x}{\delta_y}$ must equal to $\frac{x}{y}$.
    
    Liquidity provider only need to specify $\delta_x$, and $\delta_y$ is calculated automatically using the exchange rate. Liquidity provider can specify a maximum $Y$ input amount ($\check{\delta_y}$), to protect from slippage.
    \item Likewise, for $\text{RemoveLiquidity}(\delta_x, \delta_y)$, total value of funds withdrawn from asset $X$ must equal total value of funds withdrawn from asset $Y$. A minimum $Y$ output amount ($\hat{\delta_y}$) can be specified to protect from slippage.
\end{itemize}

\subsection{Uniswap State Transition Model}
{\color{blue}
We use a modified version of the state transition system originally proposed by Zhang \etal \cite{zhang2018formal} to model the Uniswap contract. We define the state of a Uniswap contract as a tuple $(e, t, l) \in \mathbb{Z}^3$, where:

\begin{description}
\item[ETH liquidity pool ($e \in \mathbb{Z}$):] Total amount of ETH deposited by fund providers, in its base unit (wei).
\item[ERC20 asset $T$ liquidity pool ($t \in \mathbb{Z}$):] Total amount of ERC20 asset $T$ deposited by fund providers, in its base unit.
\item[Asset $L$ supply ($l \in \mathbb{Z}$):] Current total supply of asset $L$. The purpose of asset $L$ is to record the contribution of each liquidity provider. When a liquidity provider deposits funds into the reserves, Uniswap will issue new asset $L$ coins as a reward. On the opposite, when funds are withdrawn, asset $L$ coins are destroyed (burnt).
\end{description}

A newly deployed Uniswap contract has state $(0, 0, 0)$. There are seven major state transition operations:

\begin{itemize}
\item $(0,0,0) \xrightarrow{\text{AddLiquidity}(\delta_e \in \mathbb{Z}, \delta_t \in \mathbb{Z})} (\delta_e, \delta_t, \delta_e)$: The first liquidity provider can set the initial exchange rate. It then deposits an equivalent value of ETH ($\delta_x$) and asset $Y$ ($\delta_y$) according to this exchange rate. Uniswap mints $\delta_x$ amount of asset $L$, and reward it to the liquidity provider.

\item $(e,t,l) \xrightarrow[(e,t,l) \neq (0,0,0)]{\text{AddLiquidity} (\delta_e \in \mathbb{Z})} (e + \delta_e, t + \lfloor \frac{\delta_e t}{e} \rfloor + 1, l + \lfloor \frac{\delta_e l}{e} \rfloor)$: Future liquidity providers add $\delta_x$ ETH and $\lfloor \frac{\delta_x y}{x} \rfloor + 1$ ERC20 asset $T$, in exchange of $\lfloor \frac{\delta_x l}{x} \rfloor$ amount of asset $L$.

\item $(e,t,l) \xrightarrow{\text{RemoveLiquidity}(\delta_l)} (e - \lfloor \frac{\delta_l e}{l}\rfloor, t - \lfloor \frac{\delta_l t}{l}\rfloor, l - \delta_l)$: Liquidity providers remove $\lfloor \frac{\delta_l x}{l}\rfloor$ of ETH and $\lfloor \frac{\delta_l y}{l}\rfloor$ of ERC20 asset $T$, by burning $\delta_l$ asset $L$.

\item $(e,t,l) \xrightarrow{\text{TransactForT}(\delta_e)} (e + \delta_e, \lfloor \frac{1000 e t}{1000e + 997\delta_e} \rfloor, l)$: Liquidity taker transacts $\delta_e$ amount of ETH for $\lfloor \frac{1000 e t}{1000e + 997\delta_e} \rfloor - t$ amount of ERC20 asset $T$.

\item $(e,t,l) \xrightarrow{\text{TransactForETH}(\delta_t)} (\lfloor \frac{1000 e t}{1000t + 997\delta_t} \rfloor, t + \delta_t, l)$: Liquidity taker transacts$\lfloor \frac{1000 e t}{1000t + 997\delta_t} \rfloor - e$ amount of ETH, for $\delta_t$ amount of ERC20 asset $T$.

\item $(e,t,l) \xrightarrow{\text{TransactForExactT}(\delta_t)} (\lfloor \frac{1000 e t}{997(t - \delta_t)} \rfloor + 1, t - \delta_t, l)$: Liquidity taker transacts $\delta_t$ amount of ERC20 token $T$ for $\lfloor \frac{1000 e t}{997(t - \delta_t)} \rfloor + 1 - e$ amount of ETH.

\item $(e,t,l) \xrightarrow{\text{TransactForExactETH}(\delta_e)} (e - \delta_e, \lfloor \frac{1000 e t}{997(e - \delta_e)} \rfloor + 1, l)$: Liquidity taker transacts $\lfloor \frac{1000 e t}{997(e - \delta_e)} \rfloor + 1 - e$ amount of ERC20 asset $T$, for $\delta_e$ amount of ETH.
\end{itemize}

Note that state transition $\textit{TransactForT}(\delta_e)$ and $\textit{TransactForExactT}(\delta_t)$ output slightly different results, even though both of them transact ETH to ERC20 asset. Consider a Uniswap contract with a state of $(1\times10^{18},\ 200\times10^{5},\ \_)$, $\textit{TransactForT}(0.01\times10^{18})$ would transact 0.01 ETH for 197.431 ERC20 asset. On the opposite, $\textit{TransactForExactT}(197\ 431)$ would transact $0.009\ 999\ 968\ 954\ 819\ 803$ amount of ETH for the same $197.431$ ERC20 asset.
}

\subsection{Uniswap Statistics}\label{sec:appendix-uniswap}

{\color{red}
We should have the following plots for the appendix and the paper:
\begin{itemize}
    \item Cumulative liquidity per coin over time, similar to https://zumzoom.github.io/analytics/uniswap/liquidity.html. We can only show the top 5 markets, and aggregate the other markets into "other"
    \item Pie chart of the top liquidity provider for the top 5 markets, similar to https://zumzoom.github.io/analytics/uniswap/providers.html
    \item Cumulative trade volume per coin over time, similar to https://zumzoom.github.io/analytics/uniswap/total\_volume.html. We can only show the top 5 markets, and aggregate the other markets into "other"
\end{itemize}
}
