# Supplementary material for: High-Frequency Trading on Decentralized On-Chain Exchanges
Source: arXiv:2009.14021 source file (2020-09-29)
Supplement: Supplementary file 2 [file appendix.tex]

% \section{Optimal Adversarial Revenue}
% In Figure~\ref{fig:optimal-attack2} we quantify the optimal adversarial revenue by an adversarial liquidity provider conducting a burger attack on Uniswap.
