# Supplementary material for: High-Frequency Trading on Decentralized On-Chain Exchanges
Source: arXiv:2009.14021 source file (2020-09-29)
Supplement: Supplementary file 3 [file appendix_experiments.tex]

\section{Detailed Experimental Results}\label{app:experiments}
\begin{landscape}
\begin{table}
\caption{Detailed results for experiments $1$ to $10$, when the adversary acts as a liquidity taker to attack another liquidity taker. Partial success denotes the attack was successful, but not all the adversarial transactions were included in the same block as the victim's transaction $T_V$.}
\label{tab:experiment_attack_1_first_10}
\tiny
% [inline block 0: 4 envs, 115082 chars -> data_tex | \begin{tabular}{lp{1.5cm}p{1.5cm}p{1.5cm}p{1.5cm}p{1.5cm}p{1.5cm}p{1.5cm}p{1.5cm}p{1.5cm}p{1.5cm}} \toprule...]

\end{table}
\end{landscape}
